# Supplementary material for: CARP: Context-Aware Reliability Prediction of Black-Box Web Services
Source: arXiv:1503.00102 source file (2018-12-30)
Supplement: Supplementary file 1 [file appendix.tex]

\vspace{1ex}
\appendix
This section provide some background of the matrix factorization model and the gradient descent algorithm, based on which we develop our \textit{CARP} approach.

\subsection{Matrix Factorization}
Matrix factorization (e.g., PMF~\cite{SalakhutdinovM07}) is a classic model to address the collaborative filtering problem, which constrains the rank of the QoS matrix, \textit{i.e.}, $rank(R) = d$. The low-rank assumption is based on the fact that the entries of $R$ are largely correlated, thereby resulting in a low effective rank in $R$. For instance, close users may have similar network conditions, and thus experience similar QoS on the same service. Concretely, factoring a matrix is to map both users and services into a joint latent factor space of a low dimensionality $d$ such that values of the user-service QoS matrix can be captured as inner products of latent factors in that space. Then the latent factors can be employed for further prediction on unknown QoS values. 

Formally, latent user factors are denoted as $U \in \mathbb{R}^{d \times n}$ and latent service factors as $S \in \mathbb{R}^{d \times m}$, which are used to fit the QoS matrix $R$, \textit{i.e.}, $R \approx U^TS$. To avoid overfitting, regularization terms that penalize the norms of the solutions (\textit{i.e.}, $U$ and $S$) are added. Thus we aim to minimize the following loss function:
\begin{equation}\label{equ:MF}
\small
\mathcal{L} = \frac{1}{2}\sum\limits_{i = 1}^n \sum\limits_{j = 1}^m I_{ij}{{(R_{ij} - U^T_i{S_j})}^2} + \frac{\lambda_U}{2}\left\| U \right\|_F^2 + \frac{\lambda_S}{2}\left\| S \right\|_F^2,
\end{equation}
where $I_{ij}$ acts as an indicator that equals to 1 if $R_{ij}$ is observed, and 0 otherwise. ${\left\|  \cdot  \right\|_F}$ denotes the \textit{Frobenius norm}~\cite{SalakhutdinovM07}, and $\lambda_U, \lambda_S$ are two parameters to control the extent of regularization.

\subsection{Gradient Descent}\label{appendix:gd}
Gradient descent is a widely used method to find a local minimum of an objective function in an iterative way. As for the PMF model expressed in Equation~\ref{equ:MF}, the gradient algorithm works by updating $U_i$ and $S_j$ simultaneously from random initialization using the following updating rules:
{\small
\begin{eqnarray}
{U_i} \leftarrow {U_i} - \eta \frac{{\partial \mathcal{L}}}{{\partial {U_i}}},\\
{S_j} \leftarrow {S_j} - \eta \frac{{\partial \mathcal{L}}}{{\partial {S_j}}},
\end{eqnarray}}
\hspace{-1.1ex}where the derivatives of $U_i$ and $S_j$ can be obtained from Equation~\ref{equ:MF} as follows:
{\small
\begin{eqnarray}
\frac{{\partial \mathcal{L}}}{{\partial {U_i}}} = \sum\limits_{j = 1}^m {{I_{ij}}(U_i^T{S_j} - {R_{ij}}){S_j} + {\lambda _U}{U_i}},\label{equ:grad1}\\
\frac{{\partial \mathcal{L}}}{{\partial {S_j}}} = \sum\limits_{i = 1}^n {{I_{ij}}(U_i^T{S_j} - {R_{ij}}){U_i} + {\lambda _S}{S_j}}\label{equ:grad2}.
\end{eqnarray}}
\hspace{-0.7ex}Hence, we derive the following updating rules:
{\small
\begin{eqnarray}
{U_i} \leftarrow {U_i} - \eta \big (\sum\limits_{j = 1}^m {{I_{ij}}(U_i^T{S_j} - {R_{ij}}){S_j} + {\lambda _U}{U_i}} \big ),\\
{S_j} \leftarrow {S_j} - \eta \big (\sum\limits_{i = 1}^n {{I_{ij}}(U_i^T{S_j} - {R_{ij}}){U_i} + {\lambda _S}{S_j}}\big ).
\end{eqnarray}}
\hspace{-0.7ex}In this way, the latent factors $U_i$ and $S_j$ move iteratively by a small step of the average gradients, \textit{i.e.}, $\frac{{\partial \mathcal{L}}}{{\partial {U_i}}}$ and $\frac{{\partial \mathcal{L}}}{{\partial {S_j}}}$, where the step size is controlled by a learning rate $\eta$. Such iterations will continue until the convergence obtained. The detailed description of the algorithm is provided in Algorithm~\ref{algo1}. 

%%%%%%%%%%%%%%%%%%%%%%%%%%%%%%%%%%%%%%%%%%%%%%%%%%
\begin{algorithm}[!b]
\caption{Gradient Descent for MF} \label{algo1}
\small
 \KwIn{The collected QoS matrix $R$, the indication matrix $I$, and the model parameters: $\eta$, $\lambda_U$ and $\lambda_S$. \tcc*[f]{$I_{ij} = 1$ if $R_{ij}$ is known; otherwise, $I_{ij} = 0$}}
 \KwOut{The QoS prediction results: $\hat{R}_{ij}$, where $I_{ij} = 0$.\vspace{1ex}}
 \SetKwBlock{Begin}{\{}{\}}
   Initialize $U \in \mathbb{R}^{d \times n}$ and $S \in \mathbb{R}^{d \times m}$ randomly\;
   \Repeat(\tcc*[f]{Batch-mode updating}){converge}{
    \ForEach(\tcc*[f]{Compute $\frac{{\partial \mathcal{L}}}{{\partial {U_i}}}$ and $\frac{{\partial \mathcal{L}}}{{\partial {S_j}}}$}){(i, j)}{    
      $\frac{{\partial \mathcal{L}}}{{\partial {U_i}}} \leftarrow \sum\limits_{j = 1}^m {{I_{ij}}(U_i^T{S_j} - {R_{ij}}){S_j} + {\lambda _U}{U_i}}$\;
      $\frac{{\partial \mathcal{L}}}{{\partial {S_j}}} \leftarrow \sum\limits_{i = 1}^n {{I_{ij}}(U_i^T{S_j} - {R_{ij}}){U_i} + {\lambda _S}{S_j}}$\;
    }
    \ForEach(\tcc*[f]{Update each $U_i$ and $S_j$}){(i, j)}{
      ${U_i} \leftarrow {U_i} - \eta \frac{{\partial \mathcal{L}}}{{\partial {U_i}}}$\;
      \vspace{0.6ex}
      ${S_j} \leftarrow {S_j} - \eta \frac{{\partial \mathcal{L}}}{{\partial {S_j}}}$\;     
        }
    }
    \BlankLine
    \ForEach(\tcc*[f]{Make prediction}){(i, j) $ \in \{I_{ij} = 0\}$}{
    $\hat{R}_{ij} = U^T_i{S_j}$\;     
    }
\end{algorithm}
%%%%%%%%%%%%%%%%%%%%%%%%%%%%%%%%%%%%%%%%%%%%%%%%%%
